# Supplementary material for: Does entanglement enhance single-molecule pulsed biphoton spectroscopy?
Source: arXiv:2307.02204 source file (2023-07-05)
Supplement: Supplementary file 1 [file appendixNPACShierarchy.tex]

\section{Asymptotic QFI Using Reduced System Dynamics : $N$-Photon Added Coherent States}\label{appendix:NPACShierarchy}

Here, will derive two-sided hierarchical master equations for $N$-photon added coherent states~(N-PACs), defined as ~\citep{zavatta2004quantum}
\begin{equation}
    \ket{\alpha,N} = \left[\int dt \xi(t) \hat{a}^{\dag}_{\mathrm{inc}}(t)\right]^N \ket{\alpha}
\end{equation}
where $\ket{\alpha}$ is a continuous mode coherent state
where the time-dependent field operator and complex amplitude are simply Fourier transforms of their frequency counterparts,
\begin{equation}
    \hat{a}(t) = \frac{1}{\sqrt{2\pi}}~\int~d\omega~e^{-i\omega t}\hat{a}(\omega), ~~\alpha(t) = \frac{1}{\sqrt{2\pi}}~\int~d\omega~e^{-i\omega t}\alpha(\omega).
\end{equation}
The action of the annihilation white noise operator on the state is the following
\begin{equation}
    \hat{a}_l(t) \ket{\alpha,N} = \sqrt{N}\xi(t)\ket{\alpha,N-1} + \alpha(t)\ket{\alpha,N},\mathrm{ ~if}~l=\mathrm{inc,~0~otherwise.}
\end{equation}
N-PACs serve as a useful middle ground between the quantum coherent Fock states and the more classical coherent pulses. Defining the analogous two-sided density operator as 
\begin{equation}
    \hat{\rho}_{\theta_1,\theta_2}^{\alpha+m,\alpha+n}(t) =  \mathrm{Tr}_{\mathrm{field}}~(~\hat{U}(t;\theta_1)\ket{\psi_0}\bra{\psi_0}\otimes\ket{\alpha,m}\bra{\alpha,n} \hat{U}^{\dag}(t;\theta_2)~)
\end{equation}
we get the following system of coupled equations
\small
\begin{align}\label{eq:hierarchyPACS}
    \frac{d}{d t}\hat{\rho}_{\theta_1,\theta_2}^{\alpha+m,\alpha+n} (t)&= -\frac{i}{\hbar}\,\left(\,\hat{H}^I_{\mathrm{matter}}(t;\theta_1)\, \hat{\rho}_{\theta_1,\theta_2}^{\alpha+m,\alpha+n}(t) - \hat{\rho}_{\theta_1,\theta_2}^{\alpha+m,\alpha+n}(t)\,\hat{H}^I_{\mathrm{matter}}(t;\theta_2)\,\right) \nonumber \\
    &+ \alpha(t)~(\hat{\rho}_{\theta_1,\theta_2}^{\alpha+m,\alpha+n}\hat{L}_{\mathrm{inc}}^{\dag}(\theta_2) -  \hat{L}_{\mathrm{inc}}^{\dag}(\theta_1) \hat{\rho}_{\theta_1,\theta_2}^{\alpha+m,\alpha+n} ) \nonumber\\
    &+ \alpha^*(t)~(\hat{L}_{\mathrm{inc}}(\theta_1)\hat{\rho}_{\theta_1,\theta_2}^{\alpha+m,\alpha+n}  - \hat{\rho}_{\theta_1,\theta_2}^{\alpha+m,\alpha+n} \hat{L}_{\mathrm{inc}}(\theta_2) )\nonumber\\
    &+ \sum_l \left( \hat{L}_l(\theta_1)\, \hat{\rho}_{\theta_1,\theta_2}^{\alpha+m,\alpha+n}(t)\, \hat{L}_l^{\dag}(\theta_2) - \frac{1}{2}\hat{L}_l^{\dag}(\theta_1)\hat{L}_l (\theta_1) \hat{\rho}_{\theta_1,\theta_2}^{\alpha+m,\alpha+n}(t) - \frac{1}{2} \hat{\rho}_{\theta_1,\theta_2}^{\alpha+m,\alpha+n}(t) \hat{L}_l^{\dag}(\theta_2)\hat{L}_l(\theta_2) \right) \nonumber\\
    &+ \sqrt{m}\xi(t)~\left(  \hat{\rho}_{\theta_1,\theta_2}^{\alpha+m-1,\alpha+n}(t)\,\hat{L}_{\mathrm{inc}}^{\dag}(\theta_2) - \hat{L}^{\dag}_{\mathrm{inc}}(\theta_1)\,\hat{\rho}^{\alpha+m-1,\alpha+n}_{\theta_1,\theta_2}(t) \right) \nonumber\\
    &- \sqrt{n}\xi^*(t)~\left(  \hat{\rho}_{\theta_1,\theta_2}^{\alpha+m,\alpha+n-1}(t)\,\hat{L}_{\mathrm{inc}}(\theta_2) - \hat{L}_{\mathrm{inc}}(\theta_1)\,\hat{\rho}^{\alpha+m,\alpha+n-1}_{\theta_1,\theta_2}(t) \right)
\end{align}
\normalsize
where we see that the master equation resembles very much the Fock master equation in Eq.~(\ref{eq:fockhierarchy}), with the addition of coherent terms, proportional to the magnitude of the coherent envelope $\alpha(t)$ that would cause coherent driving for the usual, one-sided equations of motion. The hierarchy terminates at $\hat{\rho}_{\theta_1,\theta_2}^{\alpha,\alpha}(t)$, which is simply a coherent state for which the following terminator equation holds, 
\small
 \begin{align}\ref{eq:coherentstateLindblad} 
    \frac{d}{d t}\hat{\rho}_{\theta_1,\theta_2}^{\alpha,\alpha}(t) &= -\frac{i}{\hbar}~(\hat{H}_{\mathrm{matter}}^I(t;\theta_1) \hat{\rho}_{\theta_1,\theta_2}^{\alpha,\alpha} - \hat{\rho}_{\theta_1,\theta_2}^{\alpha,\alpha} \hat{H}_{\mathrm{matter}}^I(t;\theta_2) ) \nonumber\noindent \\
    &+ \alpha(t)~~(\hat{\rho}_{\theta_1,\theta_2}^{\alpha,\alpha}\hat{L}_{\mathrm{inc}}^{\dag}(\theta_2) -  \hat{L}_{\mathrm{inc}}^{\dag}(\theta_1) \hat{\rho}_{\theta_1,\theta_2}^{\alpha,\alpha} ) + \alpha^*(t)~(\hat{L}_{\mathrm{inc}}(\theta_1)\hat{\rho}_{\theta_1,\theta_2}^{\alpha,\alpha}  - \hat{\rho}_{\theta_1,\theta_2}^{\alpha,\alpha} \hat{L}_{\mathrm{inc}}(\theta_2) )\nonumber\\
    &+ \sum_l \left( \hat{L}_l(\theta_1)\, \hat{\rho}_{\theta_1,\theta_2}^{\alpha,\alpha}(t)\, \hat{L}_l^{\dag}(\theta_2) - \frac{1}{2}\hat{L}_l^{\dag}(\theta_1)\hat{L}_l (\theta_1) \hat{\rho}_{\theta_1,\theta_2}^{\alpha,\alpha}(t) - \frac{1}{2} \hat{\rho}_{\theta_1,\theta_2}^{\alpha,\alpha}(t) \hat{L}_l^{\dag}(\theta_2)\hat{L}_l(\theta_2) \right) \nonumber\\
\end{align}
\normalsize
The initial conditions are the same as for N-photon Fock input, $\hat{\rho}_{\theta_1,\theta_2}^{\alpha+m,\alpha+n}(0) = \delta_{mn}\ket{\psi_0}\bra{\psi_0}$, where, as before, $0 \leq m,n \leq N$. Also, we note that the above equation of motion is also a standalone equation of motion for the two-sided generalised density operator for an input coherent state with envelope $\alpha(t)$, and the log-derivative of the likelihood function, which is the trace of the generalised matrix $\hat{\rho}_{\theta_1,\theta_2}^{\alpha,\alpha}(t)$, then gives the corresponding global QFI for an input coherent state.
