# Supplementary material for: Does entanglement enhance single-molecule pulsed biphoton spectroscopy?
Source: arXiv:2307.02204 source file (2023-07-05)
Supplement: Supplementary file 2 [file appendixNphotonshierarchy.tex]

\section{Asymptotic QFI Using Reduced System Dynamics : $N$-Photon Fock States}\label{appendix:fockstatehierarchy}
Incoming continuum $N$-photon Fock states~\citep{blow1990continuum} are formally constructed using the operator
\begin{equation}
    \hat{A}(\xi) = \int~ dt~\xi(t)\,\hat{a}^{\dag}(t), ~~~\mathrm{such\, that}~~ \int dt~ |\xi(t)|^2 = 1.
\end{equation}
where $\xi(t)$ is a normalised complex-valued envelope function, related to the shape of the incoming pulse, and $\hat{a}^{\dag}(t)$ is the creation operator corresponding to the incoming mode. The re-centred~(around $\omega_c$) white noise operators in Eq.~(\ref{eq:whitenoisedef}) ensure that the assumption of SVEA that went into the final form of Eq.~(\ref{eq:normalorderedSE}) is intact, so that Fourier transformed operators $\hat{a}(\omega)$ are centred around the carrier frequency $\omega_c$, and $\xi(t)$~($\xi(\omega)$) is the slowly varying envelope of the incoming state in the time~(frequency) domain.

The commutation relation $[\hat{A}(\xi),\hat{A}^{\dag}(\xi)] = 1$ holds for the envelope operator $\hat{A}(\xi)$, which can now be used to construct an $N$-photon product Fock state, each photon characterised by the envelope $\xi(t)$, as 
\begin{equation}\label{eq:xiNFockstates}
    \ket{N_\xi} = \frac{1}{\sqrt{N!}}~[\hat{A}(\xi)]^{N}\ket{0}
\end{equation}
where the normalisation follows from the commutation relation. The parametric dependence of the interaction frame Hamiltonian is embedded in the matter system operators~(assuming perfect light-matter coupling)
\begin{equation}\label{eq:apAHamiltonian}
    \hat{H}(t;\theta) = \hat{H}_{\mathrm{matter}}^I(\theta) + \hbar~(-i\hat{a}(t)\hat{L}^{\dag}(\theta) + i\hat{a}^{\dag}(t)\hat{L}(\theta))
\end{equation}
The reduced dynamics of the matter system when interacting with an initial $N$-photon Fock input of the form above, formally represented as the trace over unitary matter-field dynamics, 
\begin{equation}
     \hat{\rho}(t) = \mathrm{Tr}_{\mathrm{field}}~(~\hat{U}(t)) \ket{\psi_0}\bra{\psi_0}\otimes\ket{N_{\xi}}\bra{N_{\xi}} \hat{U}^{\dag}(t)~).
\end{equation}
(where $\ket{\psi_0}$ is the initial state of the matter state)~ can described using the hierarchical Fock master equation, obtained using Eq.~(\ref{eq:normalorderedSE}) and the input-output commutation $[\hat{a}(t),\hat{U}(t)] = \frac{1}{2}\hat{L} \hat{U}(t)$~\citep{baragiola2012n},
\begin{align}\label{eq:fockhierarchy}
    \frac{d}{d t}\hat{\rho}^{m,n}(t) &= -\frac{i}{\hbar}[\hat{H}^I_{\mathrm{matter}}(\theta),\hat{\rho}^{m,n}(t)] + \left( \hat{L}(\theta) \hat{\rho}^{m,n}(t) \hat{L}^{\dag}(\theta) - \frac{1}{2}\hat{L}^{\dag}(\theta)\hat{L}(\theta) \hat{\rho}^{m,n}(t) - \frac{1}{2}\hat{\rho}^{m,n}(t) \hat{L}^{\dag}(\theta)\hat{L}(\theta) \right)\nonumber\\
    &+ \sqrt{m}\xi(t) [\hat{\rho}^{m-1,n}(t),\hat{L}^{\dag}(\theta)] + \sqrt{n}\xi^*(t)[\hat{L}(\theta),\hat{\rho}^{m,n-1}(t)]
\end{align}
where $\hat{\rho}^{m,n}(t) = \mathrm{Tr}_{\mathrm{field}}(\hat{U}(t)\ket{\psi_0}\bra{\psi_0}\otimes\ket{m_{\xi}}\bra{n_{\xi}} \hat{U}^{\dag}(t)~), ~ \forall~ 0\leq m,n\leq N$ are the associated density operators~(ADOs). The $(N,N)$ member of the hierarchy is the reduced matter operator. Also note that the hierarchy naturally terminates at the $m=n=0$, owing to $\hat{a}_{\mathrm{inc}}(t)\ket{0}=0$. We have also utilised here the following relation,
\begin{equation}
    \hat{a}(t) \ket{N_{\xi}} = \sqrt{N}\ket{N-1_{\xi}} 
\end{equation}
obtained using the commutation relations for the white noise operators $\hat{a}(t)$, where again $\hat{L}$ is the matter dipole operator corresponding to the incoming mode of the field only. In order to solve the system of ordinary differential equations in Eq.~(\ref{eq:fockhierarchy}), we employ initial conditions $\hat{\rho}^{m,n} = \delta_{mn}\ket{\psi_0}\bra{\psi_0}$, which follows from the fact that $\mathrm{Tr}_{\mathrm{field}}\, [\ket{m_{\xi}}\bra{n_{\xi}}] = \delta_{mn}$.

We will now derive the equations of motion for the generalised density matrix $\hat{\rho}_{\theta_1,\theta_2}(T) = \mathrm{Tr}_{\mathrm{field}}\, [\hat{U}(T;\theta_1)\ket{\psi_0}\bra{\psi_0}\otimes\ket{N_\xi}\bra{N_{\xi}}\hat{U}^{\dag}(T;\theta_2)] $ for an $N$-photon Fock incoming state, by positing generalised two-sided ADOs, stated as the partial trace over field modes
\begin{equation}
   \hat{\rho}^{m,n}_{\theta_1,\theta_2}(t) =  \mathrm{Tr}_{\mathrm{field}}\,[\,\hat{U}(t;\theta_1)\,\ket{\psi_0}\bra{\psi_0}\otimes\ket{m_\xi}\bra{n_{\xi}}\,\hat{U}^{\dag}(t;\theta_2)\,].
\end{equation}
Differentiating the ADOs with respect to time yield the following generalised Fock master equations, 
\begin{align}\label{eq:hierarchyMolmer}
    \frac{d}{d t}\hat{\rho}_{\theta_1,\theta_2}^{m,n} (t)&= -\frac{i}{\hbar}\,\left(\,\hat{H}^I_{\mathrm{matter}}(t;\theta_1)\, \hat{\rho}_{\theta_1,\theta_2}^{m,n}(t) - \hat{\rho}_{\theta_1,\theta_2}^{m,n}(t)\,\hat{H}^I_{\mathrm{matter}}(t;\theta_2)\,\right) \nonumber \\
    &+ \left( \hat{L}(\theta_1)\, \hat{\rho}_{\theta_1,\theta_2}^{m,n}(t)\, \hat{L}^{\dag}(\theta_2) - \frac{1}{2}\hat{L}^{\dag}(\theta_1)\hat{L} (\theta_1) \hat{\rho}_{\theta_1,\theta_2}^{m,n}(t) - \frac{1}{2} \hat{\rho}_{\theta_1,\theta_2}^{m,n}(t) \hat{L}^{\dag}(\theta_2)\hat{L}(\theta_2) \right) \nonumber\\
    &+ \sqrt{m}\xi(t)~\left(  \hat{\rho}_{\theta_1,\theta_2}^{m-1,n}(t)\,\hat{L}^{\dag}(\theta_2) - \hat{L}^{\dag}(\theta_1)\,\hat{\rho}^{m-1,n}_{\theta_1,\theta_2}(t) \right) \nonumber\\
    &- \sqrt{n}\xi^*(t)~\left(  \hat{\rho}_{\theta_1,\theta_2}^{m,n-1}(t)\,\hat{L}(\theta_2) - \hat{L}(\theta_1)\,\hat{\rho}^{m,n-1}_{\theta_1,\theta_2}(t) \right)
\end{align}
where we have used the cyclicity of partial trace $\mathrm{Tr}_{\mathrm{B}}~[\hat{O}_{\mathrm{B}}\hat{\rho}_{AB}] = \mathrm{Tr}_{\mathrm{B}}~[\hat{\rho}_{AB}\mathrm{\hat{O}}_{\mathrm{B}}]$ as well as the commutation relation $[\hat{a},\hat{U}(t)] = \frac{1}{2}\hat{L} \hat{U}(t)$. Also, Eq.~(\ref{eq:hierarchyMolmer}) reduces to Eq.~(\ref{eq:fockhierarchy}) for $\theta_1=\theta_2$, as it should. This hierarchy of equations have the same initial and terminator conditions, so that $\hat{\rho}_{\theta_1,\theta_2}^{m,n}(0) = \delta_{mn}\ket{\psi_0}\bra{\psi_0}$, and $0\leq m,n\leq N$, again imposed by the annihilation operator $\hat{a}_l(t)$ driving vacuum to zero. The QFI of the global field-matter state is then given by the variation of the logarithm of the trace of the $\hat{\rho}_{\theta_1,\theta_2}^{N,N}(t)$ ADO, at $\theta_1=\theta_2=\theta$.

Keeping in mind the fact that $\{\ket{n}_{\xi}$\}, each element defined in the Eq.~(\ref{eq:xiNFockstates}), form a complete basis for arbitrary photon states in the temporal mode $\xi(t)$, an arbitrary $\xi$-mode $N$-photon density matrix $\hat{\rho}_{\xi} $ can be expanded as
\begin{equation}\label{eq:arbitxidensity}
    \hat{\rho}_{\xi} = \sum_{j,k = 0}^N c_{jk}\ket{j_{\xi}}\bra{k_{\xi}}.
\end{equation}
Here, $c_{jk}$ is the expansion coefficient for the the $\xi$-mode number basis element $\ket{j_{\xi}}\bra{k_{\xi}}$. The linearity of the  partial trace operation means that we can expand our hierarchical equations to the most general $\xi$-envelope propagating field. Thus, for an initial state 
\begin{equation}
   \hat{\rho}_0 = \ket{\psi_0}\bra{\psi_0}\otimes\hat{\rho}_{\xi},
\end{equation}
using the linearity of the two-sided channel in Eq.~(\ref{eq:krausgeneralizeddensity}), the final state of the matter-field state is the linear combination
\begin{align}
    \hat{\rho}_{\theta_1,\theta_2}(t) &= \sum_{j,k}~c_{jk}\, \mathrm{Tr}_{\mathrm{field}}~[\hat{U}(t;\theta_1)\ket{\psi_0}\bra{\psi_0}\otimes\ket{j_{\xi}}\bra{k_\xi}\hat{U}^{\dag}(t;\theta_2)] \nonumber\\
    &= \sum_{j,k}~ c_{j,k}\,\hat{\rho}_{\theta_1,\theta_2}^{jk}(t)
\end{align}
The elements of the above expansion $\hat{\rho}_{\theta_1,\theta_2}^{j,k}(t)$ each admit corresponding hierarchies of Eq.~(\ref{eq:hierarchyMolmer}), with the initial and terminator conditions adjusted accordingly, so that $\hat{\rho}_{\theta_1,\theta_2}^{m,n}(0) = \hat{\rho}_{\theta_1,\theta_2}^{j,k}$ and $0\leq m \leq j, ~ 0\leq n \leq k, ~\forall\, m,n$.  

\subsection{Free Space Scenario:}
So far, we have assumed perfect coupling between the matter system and the incoming light, so that there is no spontaneous decay into environmental electromagnetic modes. However, spectroscopic experiments in free space demand a treatment that includes coupling to environmental modes, which we will treat here in the context of the two-sided hierarchies for GDM for $N$-photon Fock states.

Spontaneous decay into initially unoccupied environmental EM modes can be accounted for, in terms of its effects on reduced dynamics of the rest of the system, using a single bosonic mode~\citep{Albarelli2022}. The Hamiltonian in  Eq.~(\ref{eq:apAHamiltonian}) can then be amended to be the following
\begin{equation}\label{eq:Hamiltonianamended}
    \hat{H}_{\mathrm{FS}}(t;\theta) = \hat{H}_{\mathrm{matter}}^I(\theta) + \hbar~(-i\hat{a}(t)\hat{L}_a^{\dag}(\theta) + i\hat{a}^{\dag}(t)\hat{L}_a(\theta)) + \hbar~(-i\hat{b}(t)\hat{L}_b^{\dag}(\theta) + i\hat{b}^{\dag}(t)\hat{L}_b(\theta)) 
\end{equation}
Let us now define the two-sided GDM as
\begin{equation}
    \hat{\rho}_{\theta_1,\theta_2}^{m,n}(t) = \mathrm{Tr}_a\,\left[ \hat{U}(t,\theta_1)\ket{\psi_0}\bra{\psi_0}\otimes\ket{m}_{\xi}\bra{n}\otimes\ket{0}\bra{0}\,\hat{U}^{\dag}(t,\theta_2) \right],
\end{equation}
where we note that the GDM now contains, in addition to matter DOFs, the undetected mode labelled `b'. We can obtain then following hierarchy of equations,
\begin{align}\label{eq:hierarchyMolmeramended_appendix}
    \frac{d}{d t}\hat{\rho}_{\theta_1,\theta_2}^{m,n} (t)&= -\frac{i}{\hbar}\,\left(\,\hat{H}^I_{\mathrm{matter}}(t;\theta_1)\, \hat{\rho}_{\theta_1,\theta_2}^{m,n}(t) - \hat{\rho}_{\theta_1,\theta_2}^{m,n}(t)\,\hat{H}^I_{\mathrm{matter}}(t;\theta_2)\,\right) \nonumber \\
    &+ \left( \hat{L}(\theta_1)\, \hat{\rho}_{\theta_1,\theta_2}^{m,n}(t)\, \hat{L}^{\dag}(\theta_2) - \frac{1}{2}\hat{L}^{\dag}(\theta_1)\hat{L} (\theta_1) \hat{\rho}_{\theta_1,\theta_2}^{m,n}(t) - \frac{1}{2} \hat{\rho}_{\theta_1,\theta_2}^{m,n}(t) \hat{L}^{\dag}(\theta_2)\hat{L}(\theta_2) \right) \nonumber\\
    &+ \sqrt{m}\xi(t)~\left(  \hat{\rho}_{\theta_1,\theta_2}^{m-1,n}(t)\,\hat{L}^{\dag}(\theta_2) - \hat{L}^{\dag}(\theta_1)\,\hat{\rho}^{m-1,n}_{\theta_1,\theta_2}(t) \right) \nonumber\\
    &- \sqrt{n}\xi^*(t)~\left(  \hat{\rho}_{\theta_1,\theta_2}^{m,n-1}(t)\,\hat{L}(\theta_2) - \hat{L}(\theta_1)\,\hat{\rho}^{m,n-1}_{\theta_1,\theta_2}(t) \right)\nonumber\noindent\\
    &- \frac{1}{2}\,\hat{L}_b^{\dag}(\theta_1)\hat{L}_b(\theta_1)\hat{\rho}_{\theta_1,\theta_2}^{m,n}(t) - \frac{1}{2}\hat{\rho}_{\theta_1,\theta_2}^{m,n}(t)\hat{L}_b^{\dag}(\theta_2)\hat{L}_b(\theta_2) + \hat{b}^{\dag}(t)\hat{L}_b(\theta_1)\hat{\rho}_{\theta_1,\theta_2}^{m,n}(t) + \hat{\rho}_{\theta_1,\theta_2}^{m,n}(t)\hat{L}_b^{\dag}(\theta_2)\hat{b}(t) 
\end{align}
where we note the presence of additional terms in the last line of Eq.~(\ref{eq:hierarchyMolmeramended}) -- the first of the two terms correspond to spontaneous decay, while the other two correspond to coherent exchange of excitations. The initial and terminator conditions for the hierarchy are identical to those for Eq.~(\ref{eq:molmerequation}). 
This somewhat awkward partition of the joint space is necessitated by the fact the result in Eq.~(\ref{eq:plenioreln}), which can now be used to calculate the fidelity, and hence the QFI, of the detected field states using the reduced dynamics of GDM $\hat{\rho}_{\theta_1,\theta_2}^{m,n}$. The hierarchy in Eq.~(\ref{eq:hierarchyMolmeramended}) are not as practically solvable as in Eq.~(\ref{eq:hierarchyMolmer}), owing to the fact that the GDM is defined over the joint space of the discrete matter system and the (infinite dimensional) bosonic mode of the environment. This is also apparent from the presence of the white noise field operators $\hat{b}(t)(\hat{b}^{\dag}(t))$ whose matrix representation are infinite dimensional, andd certainly not amenable to numerical solution in the general sense. However, we will note here that for incoming $N$-photon Fock state, the excitation number preserving nature of the Hamiltonian in Eq.~(\ref{eq:Hamiltonianamended}) ensures that the space of the undetected bosonic mode can be limited to an $N$-dimensional space.
