# Supplementary material for: Does entanglement enhance single-molecule pulsed biphoton spectroscopy?
Source: arXiv:2307.02204 source file (2023-07-05)
Supplement: Supplementary file 3 [file appendixPDCdescription.tex]

\section{Description of Parametric Down Converted (PDC) State}
\label{app:PDC}
The biphoton state generated at the end of low-gain type-II PDC interaction in birefringent crystals~(such as BBO or KTP cystals) that converts the classical pump photon into (signal and idler) daughter photons is obtained as the first order perturbation term,
\begin{equation}\label{eq:PDCstate}
    \ket{\Phi_{\mathrm{PDC}}} = \frac{1}{\sqrt{N_{\mathrm{PDC}}}}\,\left( \ket{0} + \int d\omega_{\mathrm{S}}\int d\omega_{\mathrm{I}}\, \Phi_{\mathrm{PDC}}(\omega_{\mathrm{S}},\omega_{\mathrm{I}})\,a_{{\mathrm{S}}}^{\dag}(\omega_{\mathrm{S}})a_{\mathrm{I}}^{\dag}(\omega_{\mathrm{I}})\ket{0}     \right),
\end{equation}
where $N_{\mathrm{PDC}}$ is the normalization factor which ensures that $\ket{\Phi_{\mathrm{PDC}}}$ is well normalized. For a more complete description of the PDC process, including in the high-gain regime, see Ref.~\cite{christ2013theory}.

The bivariate JSA $\Phi_{\mathrm{PDC}}(\omega_{\mathrm{S}},\omega_{\mathrm{I}})$  is the following product of the classical pump pulse envelope~(which is assumed to be Gaussian with spectral width given by $\sigma_p$), and the sinc phase matching function for collinear setups,
\begin{equation}\label{eq:JSA1}
     \Phi_{\mathrm{PDC}}(\omega_{\mathrm{S}},\omega_{\mathrm{I}}) = -\frac{i\alpha_{\mathrm{pump}}}{\hbar}\,\mathrm{sinc}\left( \frac{\Delta k(\omega_{\mathrm{S}},\omega_{\mathrm{I}})L}{2} \right)\,\frac{1}{\sqrt{2\pi\sigma_{p}^2}}\,e^{-(\omega_{\mathrm{S}}+\omega_{\mathrm{I}}-\omega_{\mathrm{P}})^2/2\sigma_p^2},
\end{equation}
where $\alpha_{\mathrm{pump}}/\hbar$ depends on the crystal properties~(such as crystal length $L$, and the second-order -- as PDC is a three-wave mixing process -- non-linear susceptibility $\chi^{(2)}$), as well as beam properties~(chief amongst them being the beam width that fixes the area of quantization in the paraxial description).
For simplicity, we bunch these experimental parameters together into the efficiency of the downconversion process~\cite{Schlawin2017a}.
%  Throughout the text, we assume $\alpha_{\mathrm{pump}}/\hbar=0.01$~\AK{(please change this number to value you picked)}.

The phase-matching function $\Delta k(\omega_{\mathrm{S}},\omega_{\mathrm{I}})$ can be related to the different group velocities and times of arrival of the two photons by Taylor expanding the signal/idler wavevectors around their respective central frequencies~(for which conservation of energy dictates $\bar{\omega}_{\mathrm{S}} + \bar{\omega}_{\mathrm{I}} = \omega_{\mathrm{P}}$),
\begin{equation}
    k(\omega_{\mathrm{X}}) = \bar{k}_{\mathrm{X}} + \frac{\partial k}{\partial \omega_{\mathrm{X}}} \biggr\vert_{\omega_{\mathrm{X}}=\bar{\omega}_{\mathrm{X}}}~(\omega_{\mathrm{X}}-\bar{\omega}_{\mathrm{X}}) + \dots,~~{\mathrm{X}}\,=\,{\mathrm{S}},{\mathrm{I}}.
\end{equation}
The first-order coefficient can be identified as the inverse of the wavepacket group velocity $1/v_{\mathrm{X}} = \partial k/\partial \omega_{\mathrm{X}}\vert_{\omega_{\mathrm{X}}=\bar{\omega}_{\mathrm{X}}} $.
Keeping then only the linear terms in the Taylor expansion, the phase matching function is
\begin{equation}
    \Delta k(\omega_{\mathrm{S}},\omega_{\mathrm{I}})L = \left( \frac{1}{v_{\mathrm{P}}} - \frac{1}{v_{\mathrm{S}}} \right)L\,(\omega_{\mathrm{S}}-\bar{\omega}_{\mathrm{S}}) +  \left( \frac{1}{v_{\mathrm{P}}} - \frac{1}{v_{\mathrm{I}}} \right)L\,(\omega_{\mathrm{I}}-\bar{\omega}_{\mathrm{I}}) = T_{\mathrm{S}}\,(\omega_{\mathrm{S}}-\bar{\omega}_{\mathrm{I}}) + T_{\mathrm{I}}\,(\omega_{\mathrm{I}}-\bar{\omega}_{\mathrm{I}}),
\end{equation}
where $T_{\mathrm{S}} = (1/v_{\mathrm{P}}\,-\,1/v_{\mathrm{S}})L$ is the time difference between the arrival of the wavepacket travelling at the group velocity of the pump versus that of the first photon, and similarly for $T_{\mathrm{I}}$.
The time delay between the arrival of the two photons is captured by the quantity $T_{\mathrm{qent}} = T_{\mathrm{S}} - T_{\mathrm{I}}$, henceforth referred to as the entanglement time.
In the main text
% ~\AK{(please change this according to parameters used in the data)}, 
we only study two-photon states with frequency anti-correlations~($T_{\mathrm{S}}>0,T_{\mathrm{I}}>0$), with the specific choice of $T_{\mathrm{S}} = 0.12 \,T_{\mathrm{qent}}$ and $T_{\mathrm{I}} = 1.12 \,T_{\mathrm{qent}}$.
%The entanglement time $T_{\mathrm{qent}}$ itself is varied for the purposes of the calculation of the metrological quantities between $50\,\mathrm{fs}$ and $3.0\,\mathrm{ps}$.
%The distance traversed inside the crystal is equal for both beams only for collinear PDC. To account for non-collinear propagation of the daughter photons, we use instead $T_s = (1/v_p\,-\,1/v_s)L_s$, where $L_s = L\cos\theta_s$ is the length of crystal traversed by the signal photon, and similarly for the idler photon. The entanglement time is then again $T_{\mathrm{qent}} = T_s - T_i$, which now also depends on $\theta_s$ and $\theta_i$, providing an additional degree of control over the JSA $f(\omega_s,\omega_i)$ and hence the correlations between the two photons. 
Finally, the $\mathrm{sinc}$ function can be approximates as a Gaussian~\cite{Grice2001a,kuzucu2008joint,Christ2013} ignoring their minor maxima, as
\begin{equation}
    \mathrm{sinc}\left( \frac{\Delta k(\omega_{\mathrm{S}},\omega_{\mathrm{I}})L}{2} \right) \approx \mathrm{exp}\left( -\gamma(\Delta k(\omega_{\mathrm{S}},\omega_{\mathrm{I}})L)^2\right), ~~\gamma = 0.04822.
\end{equation}
yielding a JSA that is now proportional to a two-dimensional Gaussian function,
\begin{equation}\label{eq:JSAgaussian}
    \Phi_{\mathrm{PDC}}(\omega_{\mathrm{S}},\omega_{\mathrm{I}}) \approx -\frac{i\alpha_{\mathrm{pump}}}{\hbar}\,\frac{1}{\sqrt{2\pi\sigma_p^2}}\mathrm{exp}\left(-a(\omega_{\mathrm{S}}-\bar{\omega}_{\mathrm{S}})^2 + 2b\,(\omega_{\mathrm{S}}-\bar{\omega}_{\mathrm{S}})(\omega_{\mathrm{I}}-\bar{\omega}_{\mathrm{I}}) -c(\omega_{\mathrm{I}}-\bar{\omega}_{\mathrm{I}})^2 \right)
\end{equation}
where 
\begin{align}
    a = \frac{1}{2\sigma_p^2} + \gamma T_{\mathrm{S}}^2 , ~b = \frac{1}{2\sigma_p^2} + \gamma T_{\mathrm{S}} T_{\mathrm{I}}, ~ c = \frac{1}{2\sigma_p^2} + \gamma T_{\mathrm{I}}^2. 
\end{align}
While it is always possible to (numerically) construct a Schmidt decomposition for arbitrary bivariate JSAs $\Phi(\omega_{\mathrm{S}},\omega_{\mathrm{I}})$~\citep{Lamata2005}, the approximate double Gaussian JSA in Eq.~(\ref{eq:JSAgaussian}) admits an analytical Schmidt decomposition in terms of the Hermite-Gaussian~(HG) mode functions, defined as
\begin{equation}\label{eq:hgmodedef}
    h_n(x) = \frac{1}{\sqrt{2^n n! \sqrt{\pi}}}~e^{-x^2/2}\,H_n(x)~\forall\,n\in\{0,1,\dots\}.
\end{equation}
where $H_n(x)$ is the $n$-th order Hermite polynomial. Then, using Mehler's Hermite polynomial formula~\citep{abramowitz1964handbook},
\begin{equation}\label{eq:mehler}
    \sum_{n=0}^{\infty}~\frac{\mu^n H_n(x)H_n(y) }{2^n n!} = \frac{1}{\sqrt{1-\mu^2}}\,\mathrm{exp}\left[ \frac{2\mu xy - \mu^2(x^2+y^2)}{1-\mu^2}   \right],
\end{equation}
we can express the two-dimensional Gaussian JSA as the following sum of products of univariate functions,
\begin{equation}\label{eq:schmidtJSA}
    \Phi_{\mathrm{PDC}}(\omega_{\mathrm{S}},\omega_{\mathrm{I}}) \approx \sum_{n=0}^{\infty}\,r_{n,\mathrm{PDC}}\, h_n(k_{\mathrm{S}}(\omega_{\mathrm{S}}-\bar{\omega}_{\mathrm{S}}))\,h_n(k_{\mathrm{I}}(\omega_{\mathrm{I}}-\bar{\omega}_{\mathrm{I}})),\, r_{n,\mathrm{PDC}} = -\frac{i\alpha_{\mathrm{pump}}}{\hbar}\,\sqrt{\frac{1+\mu^2}{4\sqrt{ac}\sigma_p^2}}\,\mu^n,
\end{equation}
where $k_{\mathrm{S}}$ and $k_{\mathrm{I}}$ are the projections of the elliptical JSA onto the $\omega_{\mathrm{S}}$- and $\omega_{\mathrm{I}}$-axes respectively,
\begin{equation}
    \label{eq:kappa_Schmidt}
    k_{\mathrm{S}} = \sqrt{\frac{2a(1-\mu^2)}{(1+\mu^2)}}, ~ k_{\mathrm{I}} = \sqrt{\frac{2c(1-\mu^2)}{(1+\mu^2)}},
\end{equation}
the Schmidt weight factor $\mu$ is obtained using the quadratic formula,
\begin{equation}
    \mu = \frac{-\sqrt{ac} + \sqrt{ac-b^2}}{b}.
\end{equation}
Defining PDC mode creation operators for signal and idler modes as
\begin{equation}
    h_{n,{\mathrm{S}}}^{\dag} = \int d\omega_{\mathrm{S}}\,h_n(k_{\mathrm{S}}(\omega_{\mathrm{S}}-\bar{\omega}_{\mathrm{S}}))\,a_{\mathrm{S}}^{\dag}(\omega_{\mathrm{S}}),~~h_{n,{\mathrm{I}}}^{\dag} = \int d\omega_{\mathrm{I}}\,h_n(k_{\mathrm{I}}(\omega_{\mathrm{I}}-\bar{\omega}_{\mathrm{I}}))\,a_{\mathrm{I}}^{\dag}(\omega_{\mathrm{I}}),
\end{equation}
so the bosonic commutation relations for the signal and idler operators $[h_{m,{\mathrm{S}}}^{},h_{n,{\mathrm{S}}}^{\dag}] = \delta_{mn}$,  $[h_{m,{\mathrm{I}}}^{},h_{n,{\mathrm{I}}}^{\dag}] = \delta_{mn}$ hold respectively, the approximate PDC state then has the following Schmidt form
\begin{equation}
    \ket{\Phi_{\mathrm{PDC}}} \approx \frac{1}{\sqrt{N_{\mathrm{PDC}}}}~\left(\ket{0} + \sum_{n=0}^{\infty}\,r_{n,\mathrm{PDC}}\,\,h^{\dag}_{n,{\mathrm{S}}}h^{\dag}_{n,{\mathrm{I}}}\ket{0} \right) =   \frac{1}{\sqrt{N_{\mathrm{PDC}}}} \left( \ket{0} + \sum_{n=0}^{\infty}\,r_{n,\mathrm{PDC}}\,\,\ket{h_n^{\mathrm{S}}}\ket{h_n^{\mathrm{I}}}    \right)
\end{equation}
where $\ket{h_n^{\mathrm{S}}} = h^{\dag}_{n,{\mathrm{S}}}\ket{0^{\mathrm{S}}}$~($\ket{h_n^{\mathrm{I}}} = h^{\dag}_{n,{\mathrm{I}}}\ket{0^{\mathrm{I}}}$) are $n$-mode Schmidt basis kets for the signal~(idler) photons.
Finally, if we post-select for only successful detections of the two-photon state, the biphoton PDC state becomes
\begin{equation}
    \ket{\Phi_{\mathrm{PS}}} = \sum_{n=0}^{\infty}\,\tilde{r}_{\mathrm{n,PDC}}\,\,\ket{h_n^{\mathrm{S}}}\ket{h_n^{\mathrm{I}}}, ~~\tilde{r}_{\mathrm{n,PDC}} = \frac{r_{\mathrm{n,PDC}}}{\sum_{n=0}^{\infty}\,|r_{\mathrm{n,PDC}}|^2},
\end{equation}
which has the same form as Eq.~(\ref{eq:Schmidttwinstate}).
Notice that this is equivalent to renormalizing $\Phi_{\mathrm{PDC}}(\omega_{\mathrm{S}},\omega_{\mathrm{I}})$ to be treated as a proper wavefunction, thus the efficiency parameter $\alpha_{\mathrm{pump}}$ does not enter explicitly in the description of the post-selected state.
