# Supplementary material for: Does entanglement enhance single-molecule pulsed biphoton spectroscopy?
Source: arXiv:2307.02204 source file (2023-07-05)
Supplement: Supplementary file 4 [file appendixPDCtimedomain.tex]

\section{Two-Photon PDC State in Time Domain}\label{appendix:timedomainPDC}
The two-photon PDC state can be equivalently described in the time domain by Fourier transforming the frequency-labelled creation operators as
\begin{equation}
    \hat{a}^{\dag}_x(t) = \frac{1}{\sqrt{2\pi}}\,\int d\omega\,e^{-i\omega t}\,\hat{a}_x^{\dag}(\omega), ~x = s,i
\end{equation}
which can be used to transform the PDC state as
\begin{equation}
    \ket{\psi_{\mathrm{PDC}}} = \frac{1}{\sqrt{N}}\left( \ket{0} +\int dt_s \int dt_i\left[ \frac{1}{2\pi}\int d\omega_s \int d\omega_i\,e^{-i(\omega_s t_s+\omega_i t_i)} f_{\mathrm{PDC}}(\omega_s,\omega_i) \right] \hat{a}^{\dag}(t_s)\hat{a}^{\dag}(t_i) \ket{0}  \right)
\end{equation}
so the time-axes JSA is simply the two-dimensional Fourier transform of the frequency-axes JSA,
\begin{equation}
    f_{\mathrm{PDC}}(t_s,t_i) = \frac{1}{2\pi}\int d\omega_s \int d\omega_i\,e^{-i(\omega_s t_s+\omega_i t_i)} f_{\mathrm{PDC}}(\omega_s,\omega_i).
\end{equation}
This function can be analytically evaluated for the two-photon PDC state if the frequency domain JSA $f_{\mathrm{PDC}}(\omega_s,\omega_i)$ is approximated as a double Gaussian, so it admits the analytical Schmidt decomposition in Eq.~(\ref{eq:schmidtJSA}). Keeping in mind that Hermite functions $\phi_n^G(\omega)$ are eigenfunctions of the Fourier transform, so that
\begin{equation}
    \mathcal{F}\left[\phi_n^G(k\omega);t\right] = \int \frac{d\omega}{\sqrt{2\pi}}\,e^{-i\omega t}\,\phi_n^{\mathrm{G}}(k\omega) = (-i)^n\,\phi_n^{\mathrm{G}}\left( \frac{t}{k}\right),
\end{equation}
and using the Mehler's formula in Eq.~(\ref{eq:mehler}) to sum the Fourier transformed HG mode functions, we get the following final form for the time domain JSA:
\begin{equation}\label{eq:timedomainPDC}
    f_{\mathrm{PDC}}(t_s,t_i) = - \frac{i\alpha_{\mathrm{pump}}}{\hbar}\,\frac{1}{\sqrt{\pi}}\,\frac{1+\mu^2}{1-\mu^2}\,\frac{1}{\sqrt{8ac\sigma_p^2}}\,\mathrm{exp}\left[ \frac{-2\mu t_st_i}{k_s k_i(1-\mu^2)} - \frac{1+\mu^2}{2(1-\mu^2)}\left( \frac{t_s^2}{k_s^2} + \frac{t_i^2}{k_i^2}  \right)\right].
\end{equation}
This form of the time-domain JSA $f_{\mathrm{PDC}}(t_s,t_i)$ reveals that correlations between the two photons persist in the time domain, a feature of the time-energy entanglement of the two-photon PDC states. 

Note that, following the description of entangled PDC states in Appendix \ref{appendix:PDC}, the signal/idler creation operators are assumed to be centred around their respective carrier frequencies in order to obtain Eq.~(\ref{eq:timedomainPDC}). In terms of non-centred coordinates, the time-domain PDC state can be obtained by the transformation
\begin{equation}
    \tilde{f}_{\mathrm{PDC}}(t_s,t_i) = e^{-i(\omega_{s0}t_s+\omega_{i0}t_i)}\,f_{\mathrm{PDC}}(t_s,t_i).
\end{equation}
