# Supplementary material for: Does entanglement enhance single-molecule pulsed biphoton spectroscopy?
Source: arXiv:2307.02204 source file (2023-07-05)
Supplement: Supplementary file 5 [file appendix_exponentialpulse.tex]

\section{Details of QFI Calculation for Exponentially Decaying Pulses}\label{appendix:exppulsecalculation}

The outgoing pulse amplitudes can be calculated analytically for zero detuning between TLS frequency $\omega_0$ and carrier frequency $\omega_c$,
\begin{align}\label{eq:Expmodalamps}
    \left. I_k \right\vert_{\Delta=0} &= 2\Gamma\int_0^{\infty}dt_1~\int_0^{t_1}dt_1~e^{-\Gamma(t_1-t_2)}\,g_k^{\mathrm{exp}}(t_1)g_0^{\mathrm{exp}}(t_2) \nonumber\\
    &= \frac{2\Gamma}{\Gamma\tau - 1/2}~\int_0^{\infty}dt_1~L_k\left(\frac{t_1}{\tau}\right)~[e^{-t_1/\tau} - e^{-(\Gamma+1/2\tau)t_1}] \nonumber\\
    &= \frac{2\Gamma\tau}{\Gamma\tau-1/2}\int_0^{\infty}dT L_k(T)~[e^{-T} - e^{-(\Gamma\tau+1/2)T}],~~~~T=t_1/\tau \nonumber\\
    &= (-1)^k~ 8\Gamma\tau~ (1-2\Gamma\tau)^{k-1}~(1+2\Gamma\tau)^{-k-1}, ~~~~k\in\mathcal{N}\nonumber\\
     \left. I_0 \right\vert_{\Delta=0}&= \frac{4\Gamma\tau}{1+2\Gamma\tau}.
\end{align}
Using the Laplace transform relation of WL functions, $\int_0^{\infty}dT~ T~L_k(T)e^{-sT} = -\frac{\partial}{\partial s}~\left[ \frac{1}{s}(1-\frac{1}{s})^k\right]$, the $\omega_0$-modal derivative can be calculated as
\begin{align}\label{eq:Expdelderivs}
    \left.\frac{\partial I_k}{\partial \omega_0}\right\vert_{\Delta=0} &= -i~(2\Gamma)~\int_0^{\infty}dt_1~\int_0^{t_1}dt_2~(t_1-t_2)~e^{-\Gamma(t_1-t_2)}\,g_k^{\mathrm{exp}}(t_1)g_0^{\mathrm{exp}}(t_2) \nonumber\\
    &= -i\frac{2\Gamma}{\tau}\int_0^{\infty}dt_1~e^{-(\Gamma+1/2\tau)t_1}L_k\left( \frac{t_1}{\tau}\right) ~\int_0^{t_1}dt_2~(t_1-t_2)~e^{(\Gamma-1/2\tau)t_2} \nonumber\\
    &=~ \frac{i2\Gamma\tau^2}{\Gamma\tau-1/2}~\int_0^{\infty}dT~L_k(T)~\left[ \frac{e^{-(\Gamma\tau+1/2)T}}{\Gamma\tau-1/2}  + Te^{-(\Gamma\tau+1/2)T} \right] \nonumber\\
    &=~~ i(-1)^k~ 32\Gamma\tau^2~(1-2\Gamma\tau)^{k-2}~(1+2\Gamma\tau)^{-k-2}~(2\Gamma\tau-k), ~~~ k\in\mathcal{N} \nonumber\\
     \left.\frac{\partial I_0}{\partial\omega_0}\right\vert_{\Delta=0} &= -i~~ \frac{8\Gamma\tau^2}{(1+2\Gamma\tau)^2}
\end{align}

The $\omega_0$- and $\Gamma$-modal derivatives are related as,
\begin{equation}\label{eq:ExpGamDelreln}
    \left.\frac{\partial I_k}{\partial \Gamma}\right\vert_{\Delta=0} = \frac{1}{\Gamma}~ \left. I_k \right\vert_{\Delta=0} - i\left.\frac{\partial I_k}{\partial \omega_0}\right\vert_{\Delta=0}
\end{equation}
 This gives the following form for the $\Gamma$-derivatives,
\begin{align}\label{eq:Expgamderivs}
    \left.\frac{\partial I_k}{\partial \Gamma}\right\vert_{\Delta=0} &= 8\tau~(-1)^k~(1-2\Gamma\tau)^{k-2}~(1+2\Gamma\tau)^{-k-2}~[1+4\Gamma^2\tau^2-2\Gamma\tau k], ~~k\in\mathcal{N}, \nonumber\\
     \left.\frac{\partial I_0}{\partial \Gamma}\right\vert_{\Delta=0} &= \frac{4\tau}{(1+2\Gamma\tau)^2}
\end{align}
Note that the $\Gamma$-modal derivative for $\Delta=0$ is a real number, whereas the $\omega_0$-modal derivative for $\Delta=0$ is imaginary, a feature of the the parametric dependence of the amplitudes $I_k$ on $\omega_0$ and $\Gamma$. These explicit forms for the modal amplitudes and derivatives then yield the following closed expressions for the corresponding QFI,
\begin{equation}
    \mathcal{Q}(\Gamma;\ket{\chi}\bra{\chi})\big\vert_{\Delta=0} = \mathcal{Q}(\omega_0;\ket{\chi}\bra{\chi})\big\vert_{\Delta=0}  = \frac{16\tau}{\Gamma} \frac{1}{(1+2\Gamma\tau)^2}.
\end{equation}
