# Supplementary material for: Does entanglement enhance single-molecule pulsed biphoton spectroscopy?
Source: arXiv:2307.02204 source file (2023-07-05)
Supplement: Supplementary file 8 [file appendixQFIbiphoton_explicit.tex]

\section{Explicit Expressions For Outgoing Two-Photon QFI Evaluation}\label{appendix:twinQFIdetails}

\subsection{QFI of $\ket{\Phi_{\mathrm{biph,out}}}$: } 

\noindent The derivative of the conditional state is 
\begin{equation}
    \ket{\partial_{\theta}\Phi_{\mathrm{biph,out}}} = -\frac{N_{\theta}}{2(1-N)^{3/2}}\,\sum_{m}\,r_m\ket{\phi_m^{\mathrm{S}}}\ket{\xi_m^{\mathrm{I}}} + \frac{1}{\sqrt{1-N}}\,\sum_m\,r_m\,\ket{\partial_{\theta}\phi_m^{\mathrm{S}}}\ket{\xi_m^{\mathrm{I}}}
\end{equation}
Then we can get the two terms of the pure state QFI as 
\begin{equation}
    \langle \partial_{\theta}\Phi_{\mathrm{biph,out}}|\partial_{\theta}\Phi_{\mathrm{biph,out}}\rangle = \frac{N_{\theta}^2}{4(1-N)^2} + \frac{1}{1-N}\,\sum_m\,|r_m|^2\langle \partial_{\theta} \phi_m^{\mathrm{S}} | \partial_{\theta} \phi_m^{\mathrm{S}} \rangle - \frac{N_{\theta}}{(1-N)^2}\,\sum_m\,|r_m|^2\,\mathrm{Re}\langle \phi_m^{\mathrm{S}}|\partial_{\theta}\phi_m^{\mathrm{S}}\rangle
\end{equation}
and
\begin{align}
    \langle \Phi_{\mathrm{biph,out}}|\partial_{\theta} \Phi_{\mathrm{biph,out}}\rangle &= -\frac{N_{\theta}}{2(1-N)^2}\,\sum_m\,|r_m|^2\,\langle\phi_m^{\mathrm{S}}|\phi_m^{\mathrm{S}}\rangle + \frac{1}{1-N}\,\sum_m\,|r_m|^2\,\langle\phi_m^{\mathrm{S}}|\partial_{\theta}\phi_m^{\mathrm{S}}\rangle \nonumber\noindent\\
    &= -\frac{N_{\theta}}{2(1-N)} +  \frac{1}{1-N}\,\sum_m\,|r_m|^2\,\langle\phi_m^{\mathrm{S}}|\partial_{\theta}\phi_m^{\mathrm{S}}\rangle 
\end{align}
The QFI of the conditional state is then
\begin{align}\label{eq:explicittwophotonQFI}
    \mathcal{Q}(\theta;\ket{\Phi_{\mathrm{biph,out}}}\bra{\Phi_{\mathrm{biph,out}}}) &= \cancel{\frac{N_{\theta}^2}{4(1-N)^2}} + \frac{1}{1-N}\,\sum_m\,|r_m|^2\,\langle \partial_{\theta} \phi_m^{\mathrm{S}} | \partial_{\theta} \phi_m^{\mathrm{S}} \rangle - \cancel{\frac{N_{\theta}}{(1-N)^2}\,\sum_m\,|r_m|^2\,\mathrm{Re}\langle \phi_m^{\mathrm{S}}|\partial_{\theta}\phi_m^{\mathrm{S}}\rangle}  \nonumber\noindent\\
    &- \cancel{\frac{N_{\theta}^2}{4(1-N)^2}} - \frac{1}{(1-N)^2}\left| \sum_m \, |r_m|^2\, \langle\phi_m^{\mathrm{S}}|\partial_{\theta}\phi_m^{\mathrm{S}}\rangle \right|^2 + \cancel{\frac{N_{\theta}}{(1-N)^2}\sum_m\,|r_m|^2\,\mathrm{Re}\langle\phi_m^{\mathrm{S}}|\partial_{\theta}\phi_m^{\mathrm{S}}\rangle} \nonumber\noindent\\
    &=\boxed{ \frac{1}{1-N}\,\sum_m\,|r_m|^2\,\langle \partial_{\theta} \phi_m^{\mathrm{S}} | \partial_{\theta} \phi_m^{\mathrm{S}} \rangle - \frac{1}{(1-N)^2}\left| \sum_m \, |r_m|^2\, \langle\phi_m^{\mathrm{S}}|\partial_{\theta}\phi_m^{\mathrm{S}}\rangle \right|^2}
\end{align}

\subsection{QFI of $\sigma^{\mathrm{I}}$: } 
\noindent The idler density matrix has the form
\begin{equation}
    \sigma^{\mathrm{I}} = \frac{\Gamma\Gamma_{\perp}}{N}\,\sum_{mn}\,r_m r_n\,\langle \varepsilon_n^{\mathrm{E}} | \varepsilon_m^{\mathrm{E}} \rangle\,\ket{\xi_m^{\mathrm{I}}}\bra{\xi_n^{\mathrm{I}}}
\end{equation}
Analytical QFI expressions for mixed state $\sigma^{\mathrm{I}}$ require a spectral decomposition of the density operator, which is not generally available. For our results, we will evaluate $\mathcal{Q}(\theta;\sigma^{\mathrm{I}})$ numerically -- for this purpose, we need the parametric derivative
\begin{equation}
    \frac{\partial}{\partial \theta}\,\sigma^{\mathrm{I}} = \sum_{mn}\,r_m r_n \, \frac{\partial}{\partial \theta}\,\left[ \frac{\Gamma\Gamma_{\perp}}{N} \langle \varepsilon_n^{\mathrm{E}} | \varepsilon_m^{\mathrm{E}} \rangle \right]\,\ket{\xi_m^{\mathrm{I}}}\bra{\xi_n^{\mathrm{I}}}
\end{equation}
For the TLS case, for $\theta=\omega_0$,
\begin{equation}
    \frac{\partial}{\partial \omega_0}\,\sigma^{\mathrm{I}} = -\frac{2\Gamma\Gamma_{\perp}}{N} \sum_{mn}\,r_m r_n \,\int d\omega_1\,(\omega_1-\Delta)\,\frac{\tilde{\xi_n}^{*}(\omega_1)\tilde{\xi}_m(\omega_1)}{ \left[  \frac{(\Gamma+\Gamma_{\perp})^2}{4}  + (\omega_1-\Delta)^2  \right]^2 } \,\ket{\xi_m^{\mathrm{I}}}\bra{\xi_n^{\mathrm{I}}} - \frac{N_{\omega_0}}{N}\,\sigma^{\mathrm{I}}  ,
\end{equation}    
whereas for $\theta=\Gamma$,
\begin{equation}
    \frac{\partial}{\partial \Gamma}\sigma^{\mathrm{I}} = \frac{\Gamma\Gamma_{\perp}}{N}\,\left(\frac{\Gamma+\Gamma_{\perp}}{2}\right) \sum_{mn}\,r_m r_n\,\int d\omega_1\,\frac{\tilde{\xi_n}^{*}(\omega_1)\tilde{\xi}_m(\omega_1)}{ \left[  \frac{(\Gamma+\Gamma_{\perp})^2}{4}  + (\omega_1-\Delta)^2  \right]^2 } \,\ket{\xi_m^{\mathrm{I}}}\bra{\xi_n^{\mathrm{I}}} + \left(\frac{1}{\Gamma} - \frac{N_{\Gamma}}{N}\right)\,\sigma^{\mathrm{I}}.
\end{equation}
The SLD can then be evaluated using the Lyapunov equation $L_{\theta}\sigma^{\mathrm{I}} + \sigma^{\mathrm{I}}L_{\theta} = 2\frac{\partial \sigma^{\mathrm{I}}}{\partial\theta}$, so that $\mathcal{Q}(\theta;\sigma^{\mathrm{I}}) = \mathrm{Tr}(\sigma^{\mathrm{I}}L_{\theta}^2)$.
